# Supplementary material for: Reinforcement Learning with thermal fluctuations at the nano-scale
Source: arXiv:2311.17519 ancillary file (2023-12-15)
Supplement: Supplementary file 1 [file SM_Reinforcement_Learning_with_thermal_fluctuations_at_the_nanoscale.pdf]

# Reinforcement Learning with thermal fluctuations at the nano-scale: Supplemental Material

Francesco Boccardo[1,2] and Olivier Pierre-Louis[1,*]

[1] *Institut Lumière Matière, UMR5306, Université Lyon 1 - CNRS, Villeurbanne, France*
[2] *MaLGa, Department of Civil, Chemical and Environmental Engineering, University of Genoa, Genoa, Italy*

(Dated: December 15, 2023)

## CONTENTS

I. Figures S1 to S4 2

II. RL Algorithms 6
A. RL Convergence scheme 6
B. Pseudo-codes for MCL and QL 6

III. Markov Decision Process 7

IV. Drop of efficiency for small $Fd/k_BT$ 8
A. Leading order expansion between two similar policies 8
B. Expansion for small $Fd/k_BT$ 8
C. Efficiency for an $\varepsilon$-greedy policy 9
D. Stationary probability distribution for a policy $\pi$ 10
E. Expected value of the action vectors for an $\varepsilon$-greedy policy 10

V. Transfer learning 11
A. Expansion around the optimal policy 12
B. Linear policy interpolation 14

References 15

* olivier.pierre-louis@univ-lyon1.fr

## I. FIGURES S1 TO S4

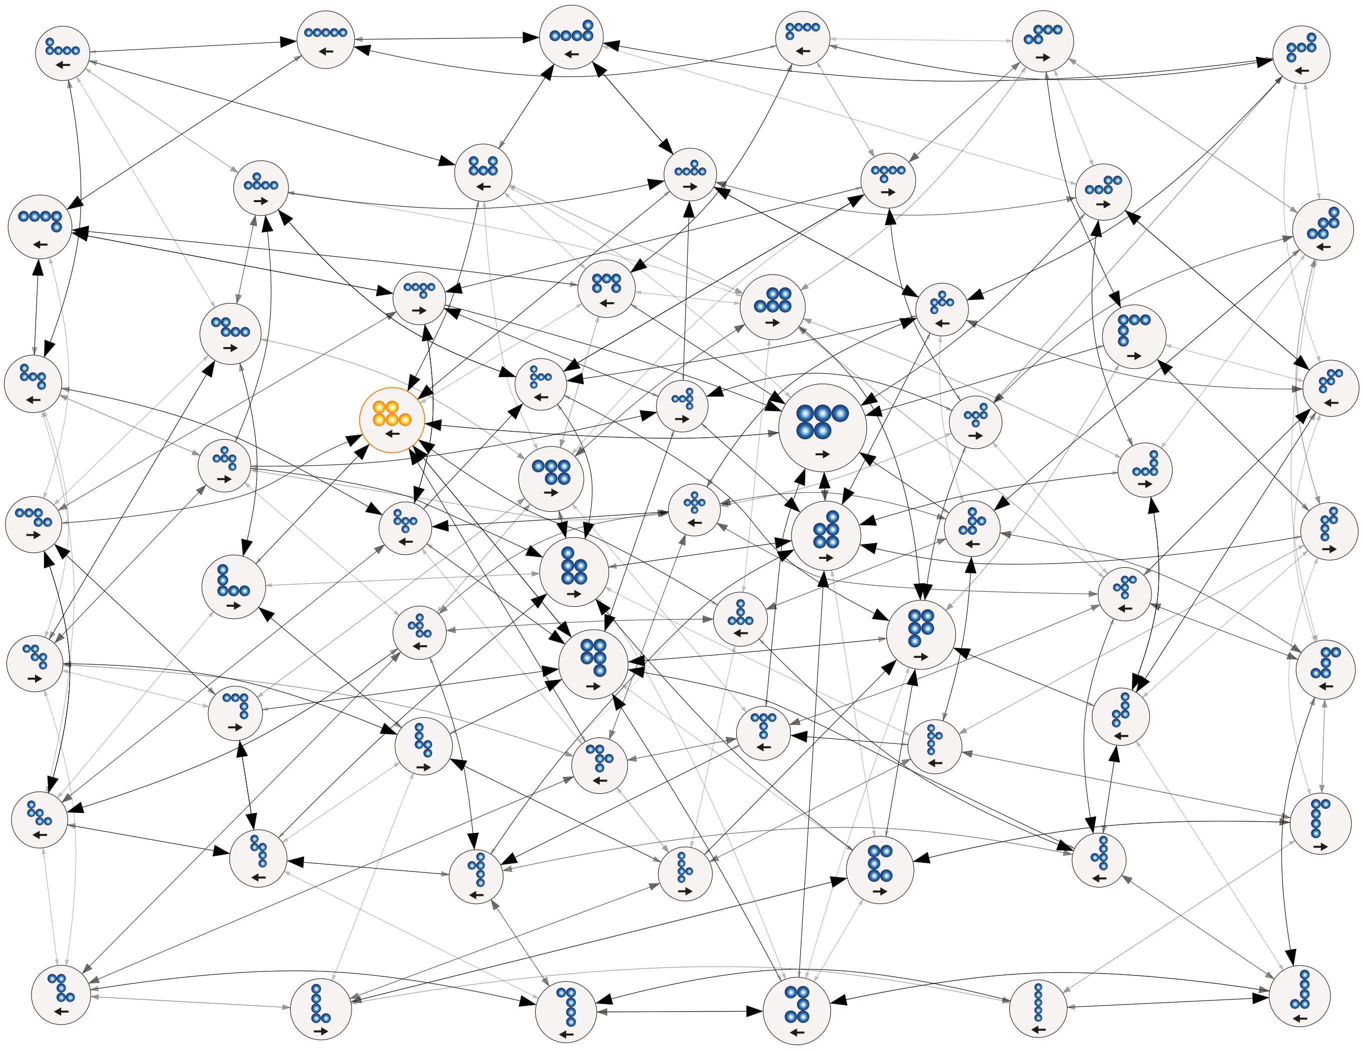

Figure S1. Graph-representation of a Markov Decision Process for a 5-particle cluster with 63 states. The size of each state is proportional to its residence time, and the width of the arrows between states are proportional to the transition probability. The yellow configuration corresponds to the target. An optimal policy for the force is represented by small arrows in the states for $J/k_BT = 4$ and $Fd/J = 0.4$.

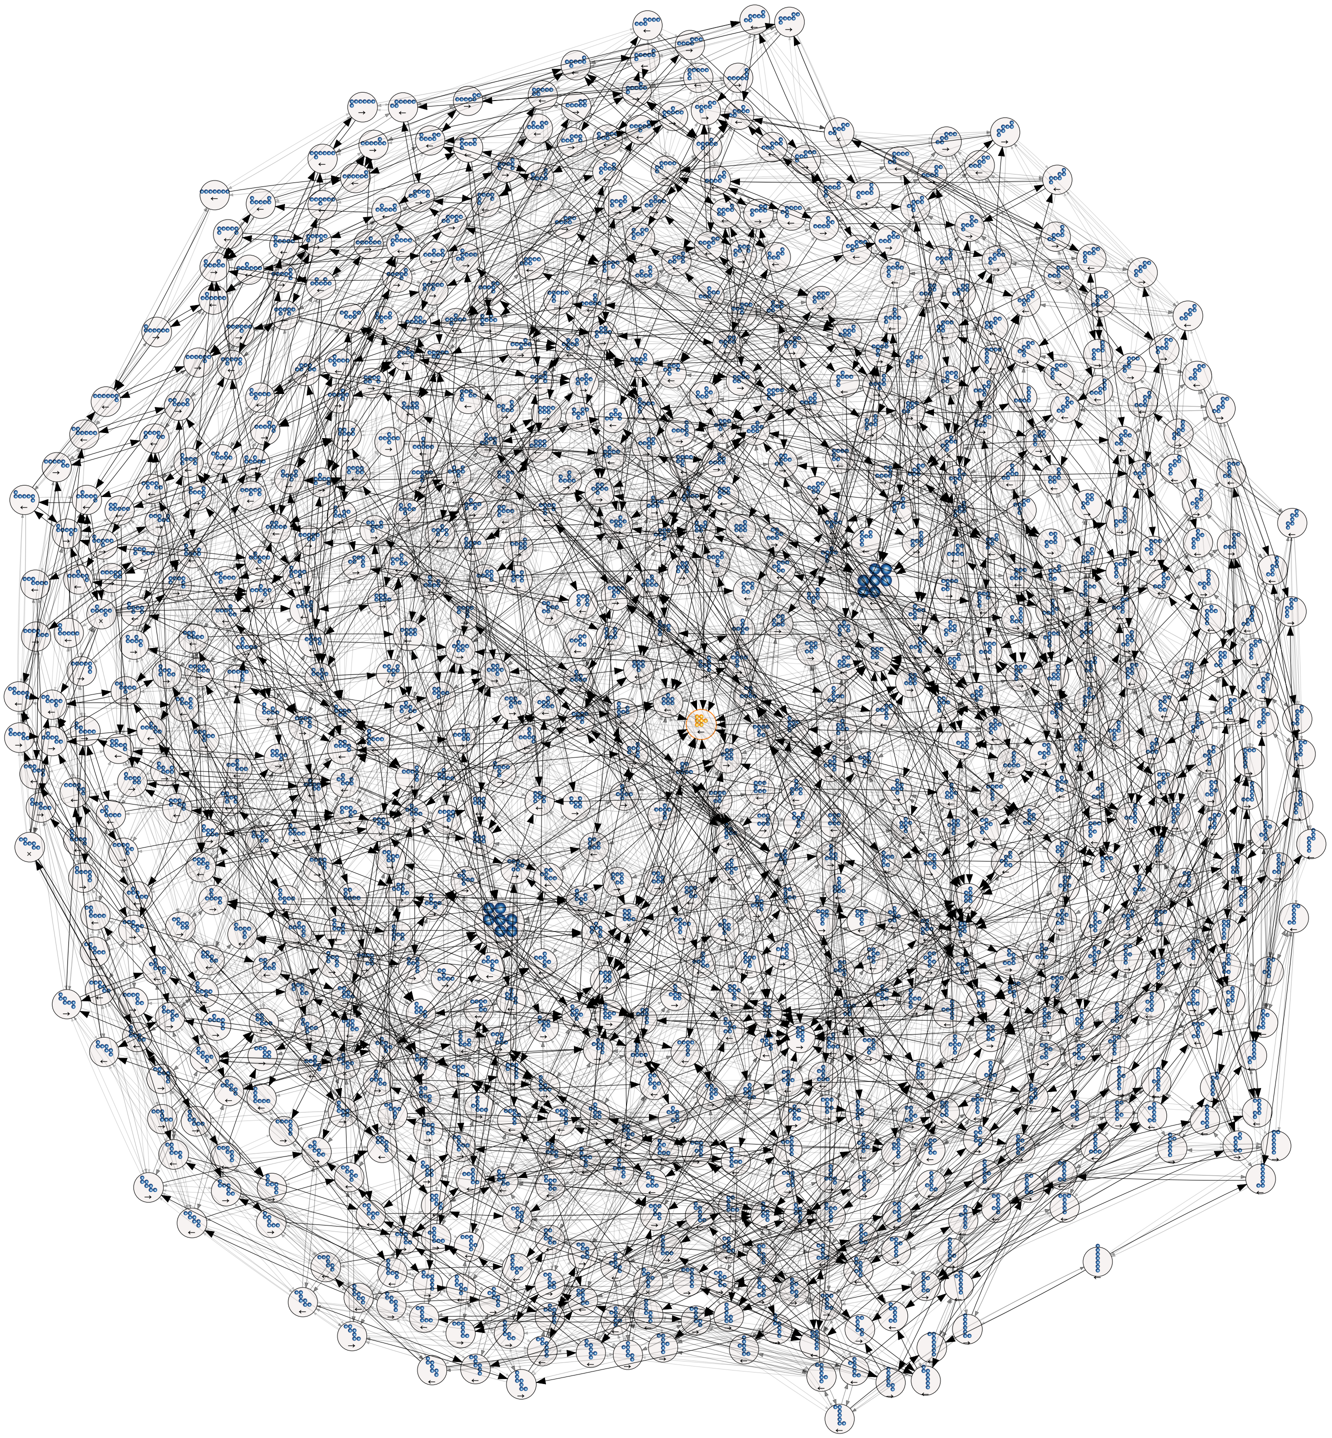

Figure S2. Graph showing the optimal policy for a 7-particle cluster with 760 states, with $J/k_BT = 5.6$ and $Fd/J = 0.4$. The yellow configuration in the center corresponds to the target.

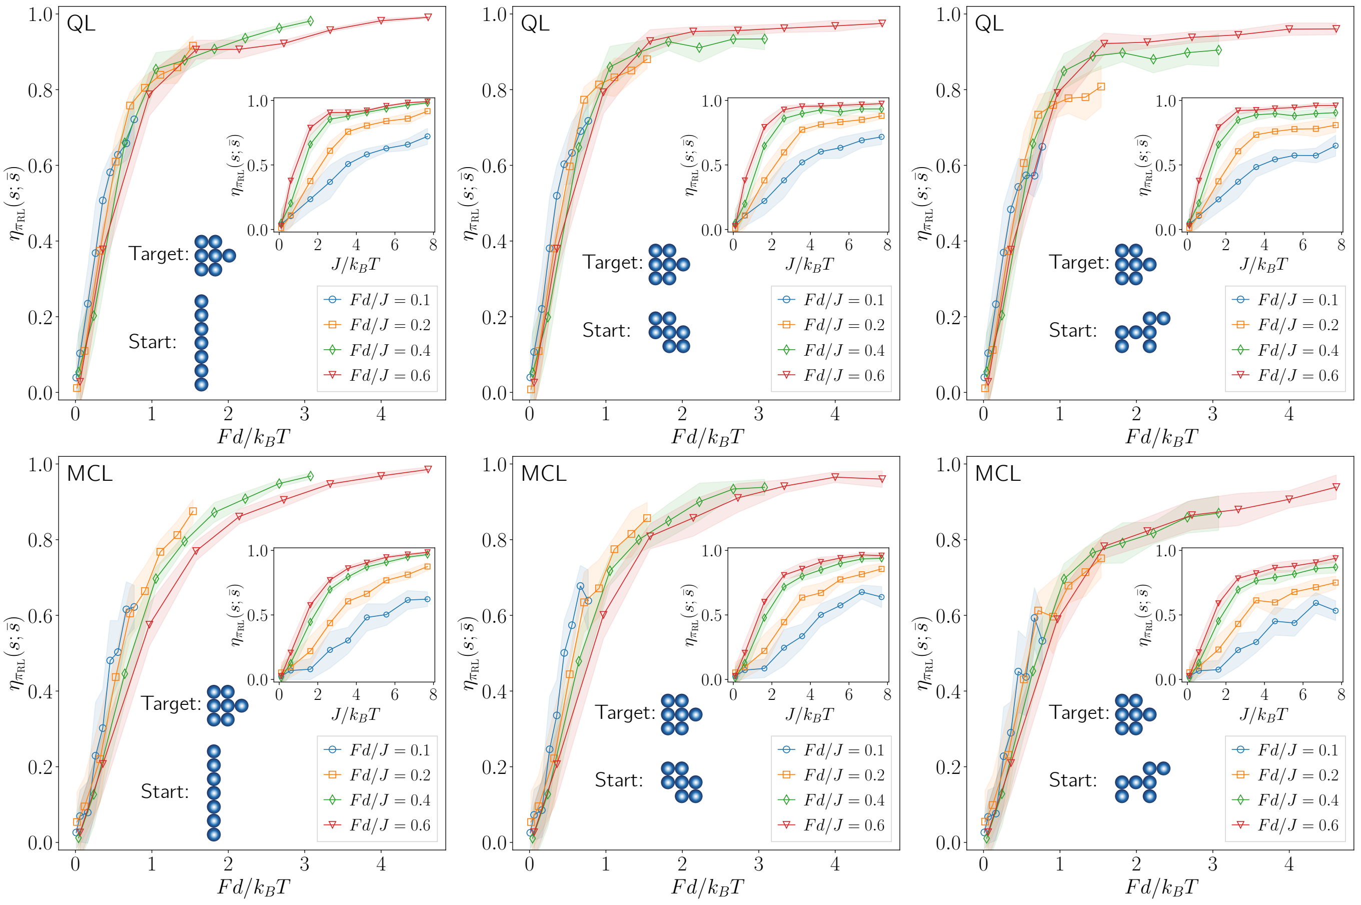


Figure S3. First passage time efficiency, defined as $\eta_{\pi_{\rm RL}}(s;\bar{s}) = (\tau_0(s;\bar{s}) - \tau_{\pi_{\rm RL}}(s;\bar{s}))/(\tau_0(s;\bar{s}) - \tau_*(s;\bar{s}))$, as a function of $Fd/k_BT$. The insets show the same results as a function of $J/k_BT$. Top row: Q-Learning (QL), bottom row: Monte Carlo Learning (MCL). A drop of efficiency at small $Fd/k_BT$ is observed, as in Fig. 2 (b,c) of the main text.

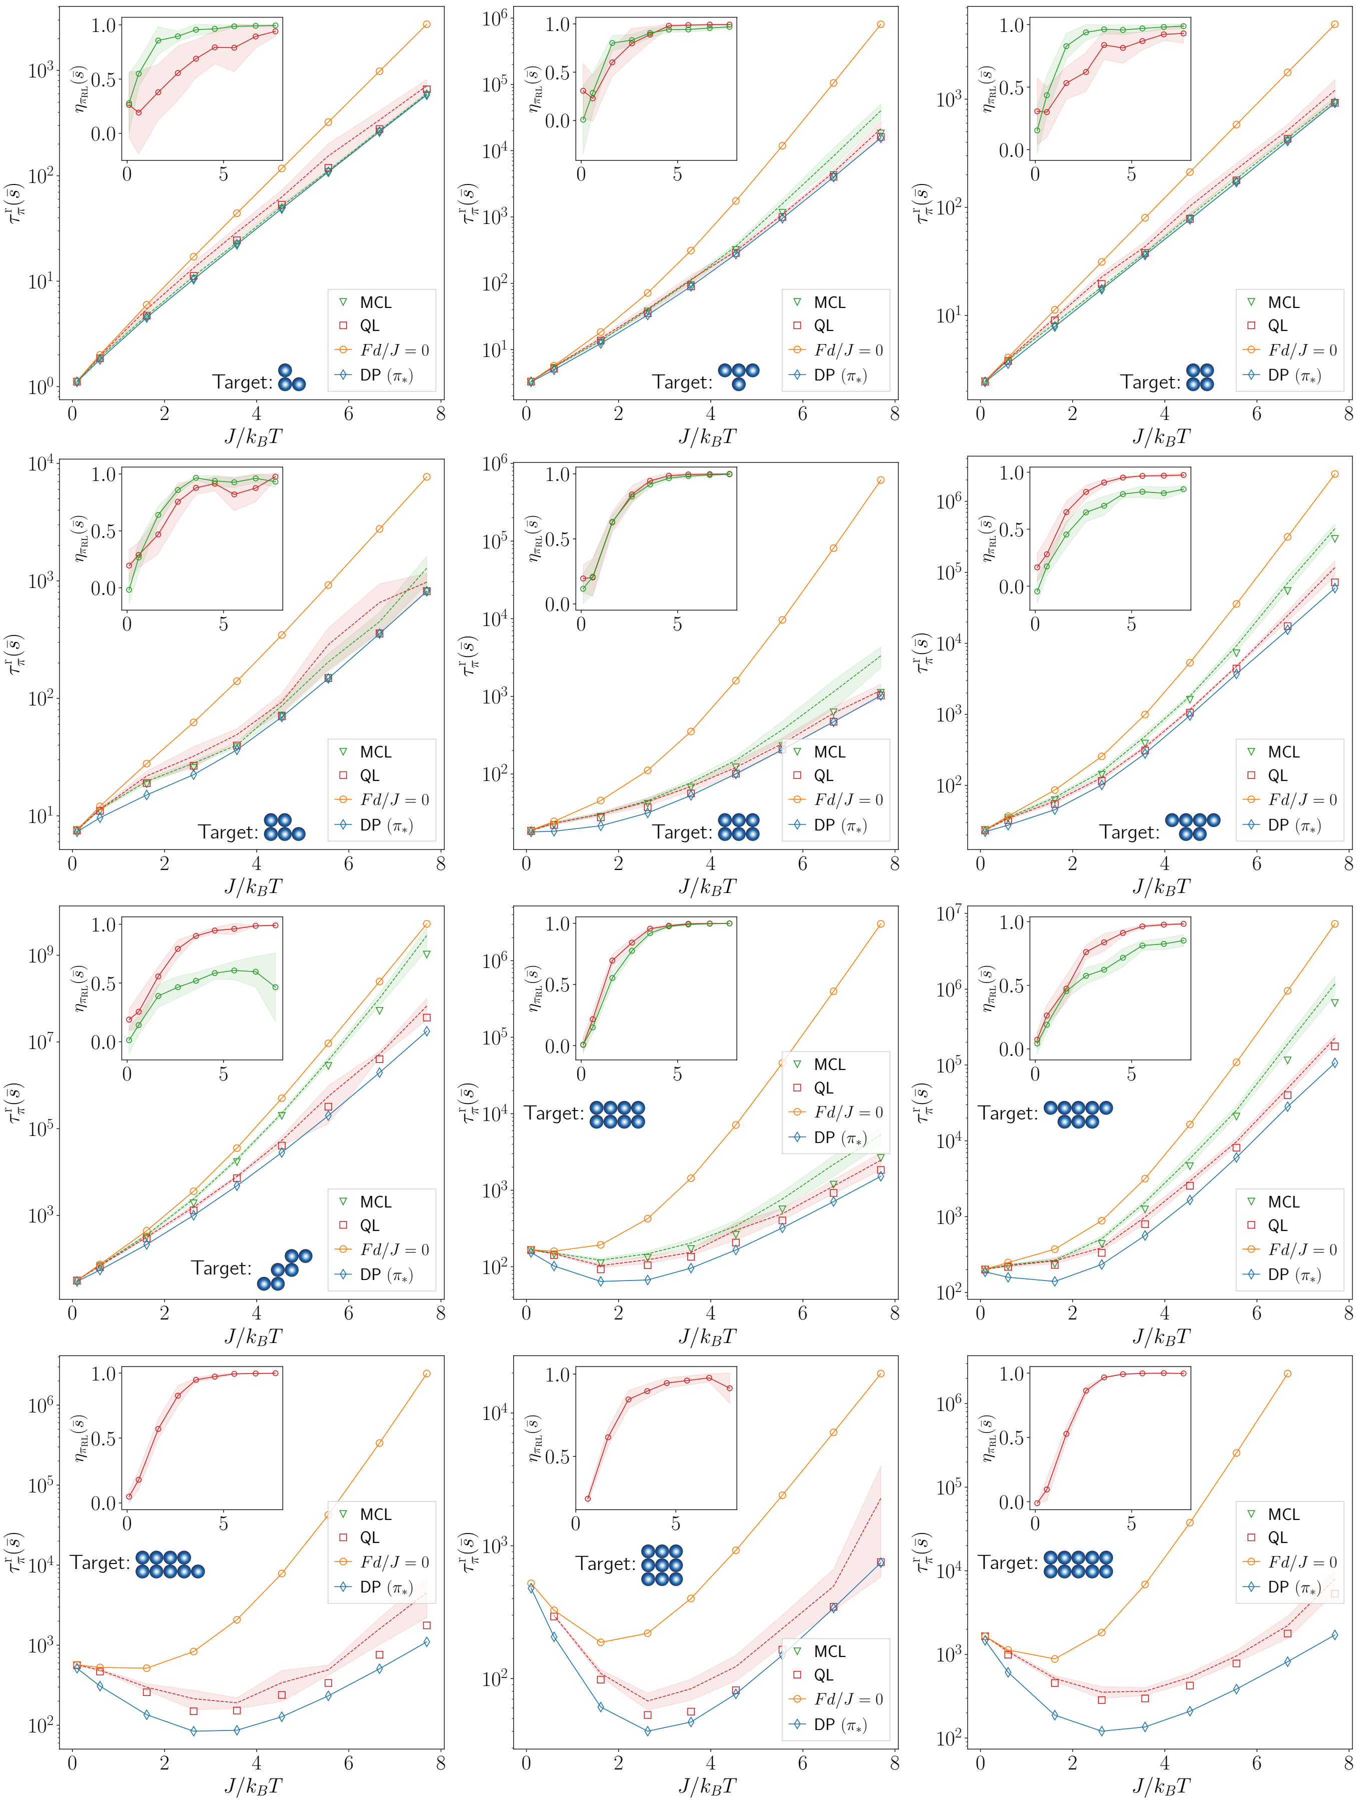


Figure S4. Return time to target as a function of $J/k_BT$ for MCL and QL, for different targets with $3 \leq N \leq 10$. The insets shows the RL efficiency. For the last three targets, only QL simulations were performed due to computational limitations.

## II. RL ALGORITHMS

### A. RL Convergence scheme

We present here the general convergence scheme we used for deciding when to stop the Reinforcement Learning (RL) tasks. The scheme is based on periodically measuring the performance of the policy learned by the RL agent using Kinetic Monte Carlo (KMC) simulations. To measure the performance of a policy $\pi$, we evaluate the expected return time to target $\tau^{\mathrm{r}}_{\pi}(\bar{s})$ and compare it with the zero-force return time to target $\tau^{\mathrm{r}}_{0}(\bar{s})$.

Because we use model-free methods, we assume no knowledge of the master equation of the system, and rely only on observations of the environment to evaluate both $\tau^{\mathrm{r}}_{\pi}(\bar{s})$ and $\tau^{\mathrm{r}}_{0}(\bar{s})$. For these evaluations, we run a KMC simulation starting from the target state $\bar{s}$ and with the force that is set according to the policy $\pi$, until we obtain a number of returns $n_{\mathrm{sam}}$ to target. The estimate of $\tau^{\mathrm{r}}_{\pi}(\bar{s})$ is obtained simply by averaging over these $n_{\mathrm{sam}}$ samples. The estimate of $\tau^{\mathrm{r}}_{0}(\bar{s})$ is obtained in the same way, but with the force set to 0. The pseudo-code of the convergence scheme is shown in Algorithm 1.

**Parameters:**
· Number of samples $n_{\mathrm{sam}}$ to evaluate the return time to target of a policy
· Number of runs $n_{\mathrm{runs}}$ that must pass without an improvement before learning is stopped
· Number of episodes $n_{\mathrm{epi}}$ of the first learning run
· Small number $I_{\mathrm{tol}}$ representing the tolerance on the improvement check

Run KMC simulation to estimate $\tau^{\mathrm{r}}_{0}(\bar{s})$ with $n_{\mathrm{sam}}$ samples
$k \leftarrow 1$
$Counter \leftarrow 0$
$I_* \leftarrow 0$
**While** $Counter < n_{\mathrm{runs}}$ **:**
  Run learning algorithm on $n_{\mathrm{epi}} \times k$ episodes, which outputs a policy $\pi$
  Run KMC simulation to estimate $\tau^{\mathrm{r}}_{\pi}(\bar{s})$ of the learned policy $\pi$ with $n_{\mathrm{sam}}$
  $I \leftarrow 1 - \tau^{\mathrm{r}}_{\pi}(\bar{s})/\tau^{\mathrm{r}}_{0}(\bar{s})$
  **If** $I > I_* \times (1 + I_{\mathrm{tol}})$ **:**
    $I_* \leftarrow I$
    $Counter \leftarrow 0$
  **Else:**
    $Counter \leftarrow Counter + 1$
  $k \leftarrow k + 1$
**Output:** $\pi \approx \pi_*$

**Algorithm 1:** Pseudo-code of the general convergence scheme for the learning tasks

The general idea of this scheme is based on measuring the *improvement factor* of the policy $I = 1 - \tau^{\mathrm{r}}_{\pi}(\bar{s})/\tau^{\mathrm{r}}_{0}(\bar{s})$. First, a KMC estimate of the zero-force return time to target $\tau^{\mathrm{r}}_{0}(\bar{s})$ is computed, which will be used as a reference. Next, an initial learning run on $n_{\mathrm{epi}}$ episodes is performed and the return time of the learned policy $\tau^{\mathrm{r}}_{\pi}(\bar{s})$ is estimated. If the improvement factor is better than the best improvement factor $I_*$ obtained during previous runs (this factor is initially set to 0), within a small tolerance $I_{\mathrm{tol}}$, then the best improvement factor is updated.

The cycle is then repeated, doubling the number of learning episodes, then tripling it, and so on. Whenever the number of runs without improvement reaches a maximum value $n_{\mathrm{runs}}$, it is considered that the learning algorithm would not benefit from a further increase in the number of episodes, and the cycle is stopped.

Each time the selected learning algorithm is called, the learning run is executed with a value of $\varepsilon$ of the $\varepsilon$-greedy policy that starts from an initial value $\varepsilon_i$ and then is linearly decreased over the course of learning, reaching a final value $\varepsilon_f$ at the last episode of the run, as illustrated schematically in Fig. S5.

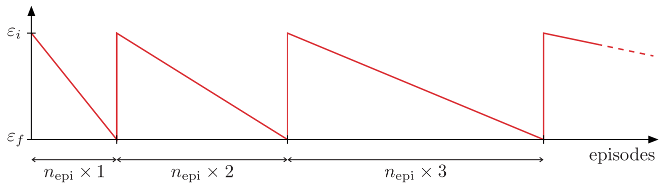


Figure S5. Schematic representation of the evolution of $\varepsilon$ over the course of the whole learning task. At the beginning of each learning run, $\varepsilon$ is reset to $\varepsilon_i$, and then decayed linearly, reaching $\varepsilon_f$ at the end of the run. At the end of each run, the performance of the policy is evaluated.

### B. Pseudo-codes for MCL and QL

We consider two tabular RL algorithms [1]: first-visit Monte Carlo Learning (MCL) and Q-Learning (QL). The pseudo-codes of these two algorithms are given in Algorithms 2 and 3.

For both algorithms, we set the discount factor $\beta = 1$ and use the following parameters for the convergence scheme: $n_{\mathrm{sam}} = 2000$, $n_{\mathrm{runs}} = 3$, $n_{\mathrm{epi}} = 1000$, $I_{\mathrm{tol}} = 0.02$. These parameters were obtained empirically from trial and error.

For MCL, we set $\varepsilon_i = 1$ and $\varepsilon_f = 0$, while for QL we set $\varepsilon_i = 1$, $\varepsilon_f = 0.1$, and the learning rate is $\alpha = 0.05$.

We also fix the maximum number of KMC moves in a single episode to $M = 10^3$, after which the episode is terminated even if the target has not been reached.

**Parameters:**
· Initial value $\varepsilon_i$ and final value $\varepsilon_f$ for $\varepsilon$
· Number of learning episodes $n_{\text{epi}}$
· Discount factor $\beta$
**Initialize:**
· $\pi \leftarrow$ an arbitrary stochastic policy
· $\hat{q}(s,a)$ arbitrarily, for all $s \in \mathcal{S}$, $a \in \mathcal{A}$
· $g\_list(s,a) \leftarrow$ empty list, for all $s \in \mathcal{S}$, $a \in \mathcal{A}$
· Decay factor $\delta\varepsilon = (\varepsilon_f - \varepsilon_i)/n_{\text{epi}}$
**Loop** for each episode **:**
  Choose $\hat{s}_0 \in \mathcal{S}$, $\hat{a}_0 \in \mathcal{A}$ randomly such that all pairs have probability $> 0$
  Generate an episode starting from $\hat{s}_0$, $\hat{a}_0$ following policy $\pi$: $\hat{s}_0, \hat{a}_0, \hat{r}_1, \ldots, \hat{s}_{K-1}, \hat{a}_{K-1}, \hat{r}_K$
  $g \leftarrow 0$
  **Loop** for each step of episode, $k = K-1, K-2, \ldots, 0$ **:**
    $g \leftarrow \beta g + \hat{r}_{k+1}$
    **If** the pair $\hat{s}_k, \hat{a}_k$ does not appear in $\hat{s}_0, \hat{a}_0, \hat{s}_1, \hat{a}_1, \ldots, \hat{s}_{K-1}, \hat{a}_{K-1}$ **:**
      Append $g$ to $g\_list(\hat{s}_k, \hat{a}_k)$
      $\hat{q}(\hat{s}_k, \hat{a}_k) \leftarrow \text{average}(g\_list(\hat{s}_k, \hat{a}_k))$
      $a^* \leftarrow \text{argmax}_a\, \hat{q}(\hat{s}_k, a)$
    For all $a \in \mathcal{A}$ :
    $$\pi(a \,|\, \hat{s}_k) \leftarrow \begin{cases} 1 - \varepsilon + \varepsilon/|\mathcal{A}| & \text{if } a = a^* \\ \varepsilon/|\mathcal{A}| & \text{if } a \neq a^* \end{cases}$$
  Decay $\varepsilon$ linearly: $\varepsilon \leftarrow \varepsilon - \delta\varepsilon$
**Output:** $\pi \approx \pi_*$

**Algorithm 2:** First-visit Monte Carlo Learning

**Parameters:**
· Initial value $\varepsilon_i$ and final value $\varepsilon_f$ for $\varepsilon$
· Number of learning episodes $n_{\text{epi}}$
· Learning rate $\alpha$
· Discount factor $\beta$
**Initialize:**
· $\pi_{\text{exp}} \leftarrow$ an arbitrary stochastic policy (used for exploration)
· $\hat{q}(s,a)$ arbitrarily, for all $s \in \mathcal{S}$, $a \in \mathcal{A}$
· Decay factor $\delta\varepsilon = (\varepsilon_f - \varepsilon_i)/n_{\text{epi}}$
**Loop** for each episode **:**
  Choose initial state $\hat{s}_0$ randomly such that all states have probability $> 0$
  **Loop** for each step of episode, up to termination **:**
    Choose action $\hat{a}$ using exploration policy $\pi_{\text{exp}}$ derived from $\hat{q}$ (e.g. $\varepsilon$-greedy)
    Take action $\hat{a}$, observe $\hat{r}$, $\hat{s}'$
    $\hat{q}(\hat{s},\hat{a}) \leftarrow \hat{q}(\hat{s},\hat{a}) + \alpha\,[\hat{r} + \beta \max_a \hat{q}(\hat{s}', a) - \hat{q}(\hat{s},\hat{a})]$
    $\hat{s} \leftarrow \hat{s}'$
  Decay $\varepsilon$ linearly: $\varepsilon \leftarrow \varepsilon - \delta\varepsilon$
**Loop** for each $s \in \mathcal{S}$ **:**
  $a^* \leftarrow \text{argmax}_a\, \hat{q}(s,a)$
  $\pi(a \,|\, s) \leftarrow \delta_{a,a^*}$
**Output:** $\pi \approx \pi_*$

**Algorithm 3:** Q-Learning

## III. MARKOV DECISION PROCESS

Consider finite discrete sets of states $\mathcal{S}$ and of actions $\mathcal{A}$. Under the action $a \in \mathcal{A}$, each possible particle move brings the cluster from state $s \in \mathcal{S}$ to state $s' \in \mathcal{S}$ with the rate $\gamma(s'|s,a)$ given by Eq. (1) of the main text (there is only one move from one state to another for clusters with more than two particles [2]). The action $a \in \mathcal{A}$ corresponds to setting the force to the value $\mathbf{F}(a) = F\mathbf{a}(a)$, where $\mathbf{a}(a)$ is a dimensionless vector. In the following we will omit the explicit dependence on $a$ and write $\mathbf{F} = F\mathbf{a}$. The actions modify the rewards via the term $\mathbf{F} \cdot \mathbf{u}d/k_BT = (\mathbf{a} \cdot \mathbf{u})Fd/k_BT$ in Eq. (1) of the main text. In our simulations, particles can move to the 8 nearest and next-nearest neighbors. Defining the unit vectors $\mathbf{e}_x$, $\mathbf{e}_y$, the products $\mathbf{u} \cdot \mathbf{e}_x$ and $\mathbf{u} \cdot \mathbf{e}_y$ take one of the three values $-d/2, 0, d/2$ depending on the direction of the move. We have performed simulations in the specific case with only three actions $a \in \mathcal{A} = \{-1, 0, 1\}$, with the corresponding action vectors $\mathbf{a} = a\mathbf{e}_x$.

Following general approaches of Markov chains, instead of considering all the Poisson processes associated to each move with its own rate, it is sufficient to consider only two processes, the time $\hat{t}$ at which the first move occurs—called the residence time—with probability $\exp[t/t(s,a)]/t(s,a)$ and the selection of the next state $s'$ with transition probability $p(s'|s,a) = \gamma(s'|s,a)t(s,a)$. Here, we have defined the average residence time

$$t(s,a) = \Big( \sum_{s' \in \mathcal{B}_s} \gamma(s'|s,a) \Big)^{-1} , \tag{1}$$

where $\mathcal{B}_s$ are the states that can be reached from $s$ in one particle move.

The transition probability and residence time under the policy $\pi(a|s)$ are defined as

$$p_\pi(s,s') = \mathbb{E}_\pi[p(s'|s,a)] = \sum_{a \in \mathcal{A}} \pi(a|s)p(s'|s,a) , \tag{2}$$

$$t_\pi(s) = \mathbb{E}_\pi[t(s,a)] = \sum_{a \in \mathcal{A}} \pi(a|s)t(s,a) . \tag{3}$$

The average first passage times $\tau_\pi(s;\bar{s})$ for reaching the target site $\bar{s}$ when starting at $s$ obey the recursion relation

$$\tau_\pi(s;\bar{s}) = t_\pi(s) + \sum_{s' \in \mathcal{B}_s} p_\pi(s,s')\tau_\pi(s';\bar{s}) , \tag{4}$$

supplemented with the boundary condition $\tau_\pi(\bar{s};\bar{s}) = 0$.

We also define the effective rates $\gamma_\pi(s,s')$:

$$\gamma_\pi(s,s') = \frac{p_\pi(s,s')}{t_\pi(s)} . \tag{5}$$

Remark that $\gamma_\pi(s,s')$ in general does not obey a relation similar to Eq. (2):

$$\gamma_\pi(s,s') \neq \mathbb{E}_\pi[\gamma(s'|s,a)] . \tag{6}$$

However, the equality holds in special cases such as deterministic policies. Another special case will be discussed below in Section IV B.

## IV. DROP OF EFFICIENCY FOR SMALL $Fd/k_BT$

### A. Leading order expansion between two similar policies

Consider the rates $\gamma(s,s')$ from state $s$ to state $s'$. For any real function $f(s)$ defined on all states $s$ we define the Laplacian-like operator

$$\Delta_\gamma f(s) = \sum_{s'\in\mathcal{B}_s} \left(\gamma(s',s)f(s') - \gamma(s,s')f(s)\right). \quad (7)$$

Remark that $\Delta_\gamma$ is not strictly speaking a Laplacian operator because it is not symmetric due to absence of $s \leftrightarrow s'$ symmetry in $\gamma(s',s)$. Consider another real function $v(s)$ defined on all states $s$. We define the auxiliary function $\tilde{v}(s)$ which is equal to $v(s)$ on all states but the target state $\bar{s}$. Then, we have

$$\sum_s f(s)\tilde{\Delta}^\dagger_\gamma v(s) = \sum_s v(s)\Delta_\gamma f(s) - \frac{f(\bar{s})}{t_\gamma(s)}(\tilde{v}(\bar{s}) - v(\bar{s}))\,, \quad (8)$$

where, unless stated otherwise, the sums over $s$ runs over the set $\mathcal{S}$ of all states and

$$t_\gamma(s) = \Big(\sum_{s'\in\mathcal{B}_s} \gamma(s,s')\Big)^{-1}, \quad (9)$$

and we have defined the modified adjoint of the Laplacian-like operator

$$\tilde{\Delta}^\dagger_\gamma v(s) = \sum_{s'\in\mathcal{B}_s} \gamma(s,s')(v(s') - \tilde{v}(s))\,. \quad (10)$$

In our problem, the Laplacian-like operator appears in the stationary master equation

$$\Delta_{\gamma_\pi} P_\pi(s) = 0\,, \quad (11)$$

where the stationary probability $P_\pi(s)$ in state $s$ obeys the normalization condition $\sum_s P_\pi(s) = 1$. A proof of Eq. (11) is provided in Section IV D. On the other hand, the adjoint operator allows for a simple rewriting of the Bellman equation Eq. (4) (see, e.g. Ref.[3])

$$\tilde{\Delta}^\dagger_{\gamma_\pi} \tau_\pi(s;\bar{s}) = -1\,, \quad (12)$$

with the usual boundary condition $\tau_\pi(s;\bar{s}) = 0$, and an additional condition for the auxiliary function $\tilde{\tau}_\pi(s;\bar{s}) = \tau^\ell_\pi(\bar{s})$, where $\tau^\ell_\pi(\bar{s}) = \tau^{\mathrm{r}}_\pi(\bar{s}) + t_\pi(\bar{s})$ is called the loop time.

Now, consider a policy $\pi_1$. In the following, the quantities evaluated with a policy will be denoted with the same index as the policy, here 1. For example $\gamma_{\pi_1}(s,s')$ will be denoted as $\gamma_1(s,s')$. Using the substitution $(\gamma,f,v) \to (\gamma_1,P_1,\tau_1)$ in Eq. (8) and using Eqs. (12) and (11), we obtain the well-known Kac relation [2, 4]

$$\tau^\ell_1(\bar{s}) = \frac{t_1(s)}{P_1(s)}\,. \quad (13)$$

If instead we consider two policies $\pi_1$ and $\pi_2$ and use the substitution $(\gamma,f,v) \to (\gamma_2,P_2,\tau_1)$ in Eq. (8), we obtain

$$\frac{\tau^\ell_1(\bar{s})}{\tau^\ell_2(\bar{s})} = -\sum_s P_2(s)\tilde{\Delta}^\dagger_{\gamma_2}\tau_1(s;\bar{s})\,. \quad (14)$$

Hence, using Eq. (12), the leading order contribution to an expansion for small $\gamma_1 - \gamma_2$ reads

$$\frac{\tau^\ell_1(\bar{s})}{\tau^\ell_2(\bar{s})} - 1 = \sum_s P_2(s)\tilde{\Delta}^\dagger_{\gamma_1-\gamma_2}\tau_2(s;\bar{s}) + O(\gamma_1-\gamma_2)^2\,. \quad (15)$$

### B. Expansion for small $Fd/k_BT$

Let us define the dimensionless parameter

$$\vartheta = Fd/k_BT\,. \quad (16)$$

The rates Eq. (1) of the main text are expanded for $\vartheta \ll 1$ as

$$\gamma(s'|s,a) = \gamma_0(s,s') + \vartheta\,\mathbf{a}\cdot\mathbf{u}_{ss'}\gamma_0(s,s') + O(\vartheta^2)\,. \quad (17)$$

As an important remark, the quantities with index 0, such as $\gamma_0(s,s')$ refer to the case with no force $F = 0$, and not to a policy with the no-force action, that would correspond to $\mathbf{a} = \mathbf{0}$.

Since the expansion Eq. (17) is linear in $\mathbf{a}$, the equality holds in Eq. (6) to linear order in $\theta$ and

$$\gamma_\pi(s,s') = \gamma_0(s,s') + \vartheta\,\mathbf{a}_\pi(s)\cdot\mathbf{u}_{ss'}\gamma_0(s,s') + O(\vartheta^2)\,, \quad (18)$$

where $\mathbf{a}_\pi(s) = \sum_a \pi(a|s)\mathbf{a}$. We then obtain two relations

$$\tilde{\Delta}^\dagger_{\gamma_1-\gamma_0}\tau_2(s;\bar{s}) = \vartheta\,\mathbf{a}_1(s)\cdot\tilde{\nabla}^\dagger_{\gamma_0}\tau_2(s;\bar{s}) + O(\vartheta^2), \quad (19)$$

$$\tilde{\Delta}^\dagger_{\gamma_1-\gamma_2}\tau_2(s;\bar{s}) = \vartheta(\mathbf{a}_1(s) - \mathbf{a}_2(s))\cdot\tilde{\nabla}^\dagger_{\gamma_2}\tau_2(s;\bar{s}) + O(\vartheta^2) \quad (20)$$

where we have defined the gradient-like operator

$$\tilde{\nabla}^\dagger_\gamma\tau(s;\bar{s}) = \sum_{s'\in\mathcal{B}_s} \mathbf{u}_{ss'}\gamma(s,s')\{\tau(s';\bar{s}) - \tilde{\tau}(s;\bar{s})\}\,. \quad (21)$$

Since $\mathbf{u}_{ss'}$ is pointing in the direction of the moves, $\tilde{\nabla}^\dagger_\gamma$ is analogous to a gradient operator. Remark that for a cluster with $N$ particles moving in two dimensions, the states $s$ can be represented as points in the $2N$ dimensional product space of the position of all particles, and the $\tilde{\nabla}^\dagger_\gamma$ operator actually acts in this high-dimensional space. Moreover, the state-to-state heterogeneity of the

weights $\gamma$ makes this gradient operator different from the naive unweighted one. This heterogeneity can be seen as a perturbation of the naive unweighted gradient definition.

Replacing $\pi_2$ by the equilibrium policy with $F = 0$ in Eq. (15) and using Eq. (19) leads to

$$\frac{\tau^{\ell}_{\pi}(\bar{s})}{\tau^{\ell}_{0}(\bar{s})} - 1 = \vartheta \sum_{s} \mathbf{a}_{\pi}(s) \cdot P_0(s) \tilde{\nabla}^{\dagger}_{\gamma_0} \tau_0(s;\bar{s}) \,, \tag{22}$$

A similar result would be obtained for any system where the actions appear via the ratio of the work of the force over the thermal energy as in Eq. (18). However if the dependence of the rates on this ratio is not exponential as in Eq. (1) of the main text, the weight of the gradient operator would be different from $\gamma_0$.

Since Eq. (22) is linear in the actions, the optimal policy is obtained as a deterministic policy with

$$a_*(s) \in \underset{a}{\operatorname{argmin}}[\mathbf{a} \cdot \tilde{\nabla}^{\dagger}_{\gamma_0} \tau_0(s;\bar{s})] \,. \tag{23}$$

Hence, the optimal action is the action that has the largest projection along the direction of the descending gradient of the first passage times without force.

In the case considered in our simulations with $\mathbf{a} = a\mathbf{e}_x$ and $a \in \{-1, 0, 1\}$, we find, when $\mathbf{e}_x \cdot \tilde{\nabla}^{\dagger}_{\gamma_0} \tau_0(s;\bar{s}) \neq 0$:

$$a_*(s) = -\operatorname{sgn}[\mathbf{e}_x \cdot \tilde{\nabla}^{\dagger}_{\gamma_0} \tau_0(s;\bar{s})] \,, \tag{24}$$

and all actions are optimal when $\mathbf{e}_x \cdot \tilde{\nabla}^{\dagger}_{\gamma_0} \tau_0(s;\bar{s}) = 0$.

### C. Efficiency for an $\varepsilon$-greedy policy

During learning, the estimate $\hat{q}(s,a)$ of the action-value function is a stochastic quantity. Its stochasticity comes from various sources of randomness in the learning process, such as the intrinsic physical noise originating in thermal fluctuations, the realizations of the choice of actions via the probabilistic policy, or some possible additional randomness in the learning algorithm (such as the random initial state in MCL and QL).

When $\vartheta = Fd/k_BT \to 0$, the rates $\gamma(s'|sa)$ can be expanded to linear order in $\vartheta$. The residence times $t(s,a)$ and the transition probabilities $p(s'|s,a)$ are then also linear in $\vartheta$. Hence, rewards $-\hat{t}$ and the returns $\hat{g}$ must also be linear in $\vartheta$, so that the RL estimate of the action-value function $\hat{q}$ is also linear in $\vartheta$:

$$\hat{q}(s,a) = \hat{q}_0(s) + \vartheta\, \mathbf{a} \cdot \hat{\boldsymbol{\theta}}(s,a) + O(\vartheta^2) \,, \tag{25}$$

where $\hat{q}_0(s)$ is a stochastic estimate of the equilibrium value function corresponding to $F = 0$, and $\hat{\boldsymbol{\theta}}(s,a)$ is stochastic vector function. Each component $\hat{\theta}_i(s,a)$ of $\hat{\boldsymbol{\theta}}(s,a)$ weights the effect of the action $a$ in state $s$.

Let us now consider an $\varepsilon$-greedy policy based on $\hat{q}$

$$\hat{\pi}(a|s) = (1-\varepsilon)\delta_{a,\operatorname{argmax}_{a'}[\hat{q}(s,a')]} + \frac{\varepsilon}{|\mathcal{A}|} \,. \tag{26}$$

With this $\varepsilon$-greedy policy, the expansion Eq. (25) implies that to leading order, the actions simply obey a random policy

$$\langle \hat{\pi}(a|s) \rangle = \pi_{\mathrm{rand}}(a|s) + O(\vartheta) \,, \tag{27}$$

where $\pi_{\mathrm{rand}}(a|s) = 1/|\mathcal{A}|$, and the notation $\langle \cdot \rangle$ accounts for an average over the realizations of the learning process. A detailed derivation of this relation together with an expression of the subdominant term are provided in Section IV E. Remark that this implies that the random policy is a consistent limit of the learned policy as $\vartheta = Fd/k_BT \to 0$. We therefore obtain the leading order expression for the expected value of the action vectors in RL

$$\langle \mathbf{a}_{\hat{\pi}}(s) \rangle = \sum_{a} \langle \hat{\pi}(a|s) \rangle\, \mathbf{a} = \frac{\sum_a \mathbf{a}}{|\mathcal{A}|} + O(\vartheta) \,. \tag{28}$$

Hence, from Eq. (22), we have

$$\begin{aligned} \frac{\langle \tau^{\ell}_{\hat{\pi}}(\bar{s}) \rangle}{\tau^{\ell}_{0}(\bar{s})} - 1 &= \vartheta \sum_{s} \langle \mathbf{a}_{\hat{\pi}}(s) \rangle \cdot P_0(s) \tilde{\nabla}^{\dagger}_{\gamma_0} \tau_0(s;\bar{s}) + O(\vartheta^2) \\ &= \frac{\tau^{\ell}_{\pi_{\mathrm{rand}}}(\bar{s})}{\tau^{\ell}_{0}(\bar{s})} - 1 + O(\vartheta^2) \,. \end{aligned} \tag{29}$$

Since the learned policy tends to a random policy as $Fd/k_BT \to 0$, the results above suggest to define of the efficiency as

$$\eta^{\ell}_{\pi}(\bar{s}) = \frac{\tau^{\ell}_{\pi_{\mathrm{rand}}}(\bar{s}) - \tau^{\ell}_{\pi}(\bar{s})}{\tau^{\ell}_{\pi_{\mathrm{rand}}}(\bar{s}) - \tau^{\ell}_{\pi_*}(\bar{s})} \,. \tag{30}$$

Using Eqs. (29) and (22), we obtain our main result:

$$\langle \eta^{\ell}_{\hat{\pi}}(\bar{s}) \rangle = O(\vartheta). \tag{31}$$

There are two differences between the definition of the efficiency Eq. (30) and the definition that we use in the main text. The first one is that we use $\tau^{\ell}_{\pi}(\bar{s})$ instead of $\tau^{\mathrm{r}}_{\pi}(\bar{s})$ which is used in simulations (as in our previous work Ref. [5]). In general, using the Kac relation Eq. (13), the relative error of this assumption is: $(\tau^{\ell}_{\pi}(\bar{s}) - \tau^{\mathrm{r}}_{\pi}(\bar{s}))/\tau^{\ell}_{\pi}(\bar{s}) = P_{\pi}(\bar{s})$. As discussed in details in Ref. [2], this relative difference is usually very small, and can be significant only at low temperatures when $\bar{s}$ is a unique ground state, or when the cluster only has 2 or 3 particles.

The second difference is the use the zero-force policy in Eq. (4) of the main text as a reference instead of the random policy in Eq. (30). We have seen above that the random policy is a consistent definition of the policy in the limit $\vartheta = Fd/k_BT \to 0$. The difference between the return times of random and zero-force policies is small as discussed in the Supplemental Material of Ref. [5], and due to the linearity in the actions in Eq. (22), this difference vanishes as $\vartheta \to 0$ if

$$\sum_{a} \mathbf{a} = \mathbf{0} \,, \tag{32}$$

which is the case in our simulations. In practice, this condition is convenient to avoid any bias in the average force associated to a random choice of the actions.

Thus, the two definitions of the efficiency lead to very similar results, and we can assume that $\eta_\pi^\ell(\bar{s}) \approx \eta_\pi(\bar{s})$, so that $\langle \eta_\pi(\bar{s}) \rangle = O(\vartheta)$ from Eq. (31).

### D. Stationary probability distribution for a policy $\pi$

Consider a policy $\pi(a|s)$. To obtain a description that is compatible with Markov chains, we resort to an augmented state space, where states now correspond to the couple $(s,a)$ instead of $s$. Hence, we now have $|\mathcal{S}| \times |\mathcal{A}|$ states. The transition rate from $(s,a)$ to $(s',a')$ obeys

$$\gamma(s',a'|s,a) = \gamma(s'|s,a)\pi(a'|s'), \tag{33}$$

and the master equation for the time-dependent probability $P_\pi(s,a,t)$ of state $(s,a)$ reads:

$$\partial_t P_\pi(s,a,t) = \sum_{s' \in \mathcal{B}_s} \sum_{a'} \{\gamma(s,a|s',a')P_\pi(s',a',t) - \gamma(s',a'|s,a)P_\pi(s,a,t)\}. \tag{34}$$

Using these expressions and the normalization condition $\sum_a \pi(a|s) = 1$, we obtain

$$\partial_t P_\pi(s,a,t) = \pi(a|s) \sum_{s' \in \mathcal{B}_s} \sum_{a'} \gamma(s|s',a')P_\pi(s',a',t) - \frac{P_\pi(s,a,t)}{t(s,a)}, \tag{35}$$

where the residence time $t(s,a)$ is defined as

$$t(s,a) = \frac{1}{\sum_{s' \in \mathcal{B}_s} \gamma(s'|s,a)}. \tag{36}$$

Hence, the time-independent stationary distribution $P_\pi(s,a)$ obeys

$$P_\pi(s,a) = \pi(a|s)t(s,a)C_\pi(s), \tag{37}$$

where the action-independent function $C_\pi(s)$ is defined as

$$C_\pi(s) = \sum_{s' \in \mathcal{B}_s} \sum_{a'} \gamma(s|s',a')P_\pi(s',a'). \tag{38}$$

Inserting Eq. (37) in Eq. (38), and using the definition of the transition probability $p(s'|s,a) = t(s,a)\gamma(s'|s,a)$, and the transition probability for the policy $\pi$

$$p_\pi(s,s') = \sum_a \pi(a|s)p(s'|s,a), \tag{39}$$

we obtain

$$C_\pi(s) = \sum_{s' \in \mathcal{B}_s} p_\pi(s',s)C_\pi(s'). \tag{40}$$

Now defining the probability $P_\pi(s)$ as

$$P_\pi(s) = \sum_a P_\pi(s,a), \tag{41}$$

and using Eq. (37), we have

$$P_\pi(s) = \sum_a \pi(a|s)t(s,a)C_\pi(s) = t_\pi(s)C_\pi(s). \tag{42}$$

Combining Eqs. (40) and (42) and using the normalization condition $\sum_{s' \in \mathcal{B}_s} p_\pi(s,s') = 1$, we finally obtain

$$0 = \sum_{s' \in \mathcal{B}_s} \left\{ \frac{p_\pi(s',s)}{t_\pi(s')} P_\pi(s') - \frac{p_\pi(s,s')}{t_\pi(s)} P_\pi(s) \right\}, \tag{43}$$

which may be re-written as Eq. (11).

### E. Expected value of the action vectors for an $\varepsilon$-greedy policy

We assume that the stochasticity of the learning process leads to the distribution $P_{\mathrm{RL}}(q|s,a)$ for $\hat{q}$, and to the joint distribution $P_{RL1}(q_0,\boldsymbol{\theta}|s,a)$ for $\hat{q}_0$ and $\hat{\boldsymbol{\theta}}$. Since $q$, $q_0$, and $\boldsymbol{\theta}$ are related via Eq. (25), we have to linear order in $\vartheta = Fd/k_BT$

$$P_{\mathrm{RL}}(q|s,a) = \int_{-\infty}^{+\infty} \mathrm{d}\theta \; P_{RL1}(q - \vartheta \mathbf{a}\cdot\boldsymbol{\theta} + O(\vartheta^2), \boldsymbol{\theta}|s,a). \tag{44}$$

where $\mathrm{d}\theta = \prod_i \mathrm{d}\theta_i$, where $\theta_i$ is the $i$-th component of $\boldsymbol{\theta}$.

An expansion to leading order in $Fd/k_BT$ leads to

$$P_{\mathrm{RL}}(q|s,a) = P_{RL0}(q|s) - \vartheta \mathbf{a} \cdot \int_{-\infty}^{+\infty} \mathrm{d}\theta \, \boldsymbol{\theta} \, \partial_{q_0} P_{RL1}(q,\boldsymbol{\theta}|s,a) + O(\vartheta^2), \tag{45}$$

where

$$P_{RL0}(q_0|s) = \int_{-\infty}^{+\infty} \mathrm{d}\theta \; P_{RL1}(q_0, \boldsymbol{\theta}|s, a)\,. \tag{46}$$

Since $\hat{q}_0(s)$ is independent of the action in Eq. (25), $P_{RL0}(q_0|s)$ is independent of the variable $a$.

Note that since the probability distributions $P_{RL0}(q_0|s)$ and $P_{RL\theta}(q_0, \theta|s, a)$ result from the learning process, they could both depend on $\vartheta = Fd/k_BT$. Hence, they should also be expanded to linear order in $\vartheta$. However, these corrections only contribute to higher order terms in the results below, so we will not make them explicit to keep the notations simple.

The probability that the action $a$ provides the largest value of $\hat{q}$ reads

$$\mathrm{Proba}\Big\{a = \underset{a'}{\mathrm{argmax}}[\hat{q}(s,a')]\Big\} = \int_{-\infty}^{+\infty} \mathrm{d}q \, P_{\mathrm{RL}}(q|s,a) \prod_{a' \neq a} \int_{-\infty}^{q} \mathrm{d}q' P_{\mathrm{RL}}(q'|s,a')\,, \tag{47}$$

Using Eq. (45), we have to linear order in $Fd/k_BT$

$$\begin{aligned}
&\int_{-\infty}^{+\infty} \mathrm{d}q \, P_{\mathrm{RL}}(q|s,a) \prod_{a' \neq a} \int_{-\infty}^{q} \mathrm{d}q' P_{\mathrm{RL}}(q'|s,a') \\
&= \int_{-\infty}^{+\infty} \mathrm{d}q \, P_{RL0}(q|s) \left( \int_{-\infty}^{q} \mathrm{d}q' P_{RL0}(q'|s) \right)^{|\mathcal{A}|-1} \\
&- \vartheta \, \mathbf{a} \cdot \int_{-\infty}^{+\infty} \mathrm{d}q \int_{-\infty}^{+\infty} \mathrm{d}\theta \, \boldsymbol{\theta} \, \partial_q P_{RL1}(q, \theta|s) \left( \int_{-\infty}^{q} \mathrm{d}q' P_{RL0}(q'|s) \right)^{|\mathcal{A}|-1} \\
&- \vartheta \sum_{a' \neq a} \mathbf{a}' \cdot \int_{-\infty}^{+\infty} \mathrm{d}q \, P_{RL0}(q|s) \int_{-\infty}^{q} \mathrm{d}q' \int_{-\infty}^{+\infty} \mathrm{d}\theta \, \boldsymbol{\theta} \, \partial_{q'} P_{RL1}(q', \theta|s, a') \left( \int_{-\infty}^{q} \mathrm{d}q' P_{RL0}(q'|s) \right)^{|\mathcal{A}|-2} + O(\vartheta^2) \\
&= \frac{1}{|\mathcal{A}|} - \vartheta \frac{1}{|\mathcal{A}|-1} \sum_{a'} (\mathbf{a} \cdot \mathbf{J}_{\mathrm{RL}}(s,a) - \mathbf{a}' \cdot \mathbf{J}_{\mathrm{RL}}(s,a')) + O(\vartheta^2)\,,
\end{aligned} \tag{48}$$

where

$$\mathbf{J}_{\mathrm{RL}}(s,a) = -\int_{-\infty}^{+\infty} \mathrm{d}q \int_{-\infty}^{+\infty} \mathrm{d}\theta \, \boldsymbol{\theta} \, P_{RL1}(q, \theta|s, a) \partial_q \left( \int_{-\infty}^{q} \mathrm{d}q' P_{RL0}(q'|s) \right)^{|\mathcal{A}|-1}. \tag{49}$$

Hence, for an $\varepsilon$-greedy policy, one has

$$\begin{aligned}
\langle \hat{\pi}(a|s) \rangle &= (1-\varepsilon) \left\langle \delta_{a, \mathrm{argmax}_{a'}[\hat{q}(s,a')]} \right\rangle + \frac{\varepsilon}{|\mathcal{A}|} \\
&= (1-\varepsilon) \mathrm{Proba}\Big\{a = \underset{a'}{\mathrm{argmax}}[\hat{q}(s,a')]\Big\} + \frac{\varepsilon}{|\mathcal{A}|} \\
&= \frac{1}{|\mathcal{A}|} - \vartheta \frac{1-\varepsilon}{1-|\mathcal{A}|^{-1}} \sum_{a'} (\mathbf{a} \cdot \mathbf{J}_{\mathrm{RL}}(s,a) - \mathbf{a}' \cdot \mathbf{J}_{\mathrm{RL}}(s,a')) + O(\vartheta^2)\,,
\end{aligned} \tag{50}$$

where the average over the stochasticity of the learning process is denoted by the brackets $\langle \cdot \rangle$. We now evaluate the expected value of the actions on state $s$ during the learning with an $\varepsilon$-greedy policy

$$\begin{aligned}
\langle \mathbf{a}_{\hat{\pi}}(s) \rangle &= \sum_a \langle \hat{\pi}(a|s) \rangle \, \mathbf{a} \\
&= \frac{\sum_a \mathbf{a}}{|\mathcal{A}|} - \vartheta \frac{1-\varepsilon}{1-|\mathcal{A}|^{-1}} \sum_a \mathbf{a} \cdot \mathbf{J}_{\mathrm{RL}}(s,a) \left( \mathbf{a} - \frac{\sum_{a'} \mathbf{a}'}{|\mathcal{A}|} \right) + O(\vartheta^2)\,.
\end{aligned} \tag{51}$$

## V. TRANSFER LEARNING

To discuss how policies change with temperature, we use a similarity measure $\sigma$ between two policies, which decreases from 1, when they are identical, to 0, when they are uncorrelated. For deterministic policies $\pi_1$ and $\pi_2$,

respectively setting the actions $a_1(s)$ and $a_2(s)$ in state $s$, the similarity is defined as

$$\sigma[\pi_1, \pi_2 : \omega] = \sum_s \frac{\delta_{a_1(s),a_2(s)} - 1/|\mathcal{A}|}{1 - 1/|\mathcal{A}|} \frac{\omega(s)}{\sum_{s'} \omega(s')}, \quad (52)$$

where $\omega(s)$ is a weight that accounts for the relevance of state $s$, $|\mathcal{A}|$ is the total number of actions, and the Kronecker delta function $\delta_{a_1(s),a_2(s)}$ is equal to 1 when $a_1(s) = a_2(s)$ and 0 otherwise. For two optimal policies $\pi_{1*}$ and $\pi_{2*}$ obtained with DP at temperatures $T_1$ and $T_2$, the unweighted similarity $\sigma[\pi_{1*}, \pi_{2*} : 1]$ with $\omega(s) = 1$ in all states decreases from 1 to about 0.3 when $|T_2 - T_1|$ increases, as shown in Fig. S7 (a).

To have a more refined view on the changes in the policy, we define a ring as the set of states that can be reached in a minimum number of $m$ moves from the target, with $m$ the ring index [6]. A schematic of the first rings is shown in Fig. S6. As seen in Fig. S7 (b), the unweighted similarity between high- and low-temperature policies within a given ring is on average higher in rings with low $m$. To understand these smaller changes at low $m$, the first passage time averaged within each ring is plotted as a function of $m$ in Fig. S8 (a). We observe an increasing gradient as one gets closer to the target. The optimal policy is naively expected to be in the direction of descending first-passage-time gradients to bias the random walk in configuration space towards the target (as demonstrated in Section IV B). However, the average gradient direction towards the target is locally perturbed by the variability of the rates $\gamma$ from state to state. Since the gradient is on average larger at low $m$, its direction—which controls the optimal policy—will resist better to these perturbations.

Moreover, states with low ring index are intuitively expected to be important for the efficiency because the system necessarily has to go through them to reach the target. To compare the importance of different states for the efficiency we define the sensitivity

$$\chi_*(s; \bar{s}) = \frac{\mathbb{E}_{\pi_*}[q_{\pi_*}(s, a; \bar{s})] - \mathbb{E}_{\pi_{\rm rand}}[q_{\pi_*}(s, a; \bar{s})]}{\tau^{\rm r}_{\pi_*}(s)}, \quad (53)$$

where $\pi_{\rm rand}$ is a random policy. Note that $\mathbb{E}_{\pi_*}[q_{\pi_*}(s, a; \bar{s})] = -\tau_*(s, \bar{s})$. The pertinence of the sensitivity is seen from the approximate expression of the efficiency for a policy $\pi_1$ evaluated at $T_2$:

$$\eta_{\pi_1}(\bar{s})|_{T_2} \approx \sigma[\pi_1, \pi_{2*} : \chi_{2*}], \quad (54)$$

where $\chi_{2*}$ denotes $\chi_*$ for the optimal policy $\pi_{2*}$ at $T = T_2$. A derivation of this relation for $Fd/k_BT \ll 1$ is presented in Section V B. In the case $T_1 = T_2 = T$, with $\pi_{2*}$ obtained from DP and $\pi_1$ from QL, Fig. S8 (b) and Fig. S9 show that the two quantities in Eq. (54) are well correlated at small $Fd/k_BT$, and some correlation is still observed with

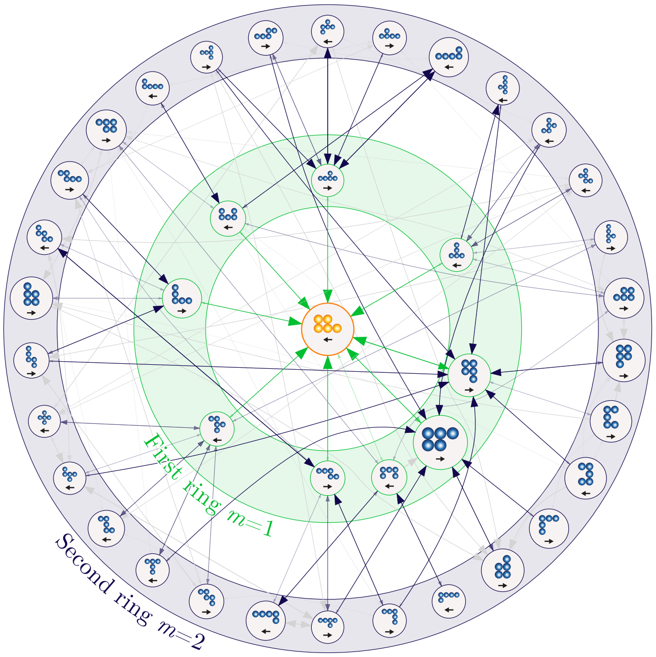


Figure S6. First two rings for a 5-particle target. The other rings with $m \geq 3$ are not shown. The full graph representation of the Markov Decision Process, with the optimal policy for the same target, is reported in Fig. S1.

a nonlinear but monotonous relation for finite $Fd/k_BT$. From Eq. (54), the efficiency of a policy $\pi_1$ learned at some temperature $T_1$ is efficient at temperature $T_2$ if it is similar to the optimal policy $\pi_{2*}$ at $T_2$ in states where the sensitivity $\chi_{2*}$ is large. Thus, $\chi_{2*}$ measures the relevance of the states for the efficiency.

Furthermore, $\chi_{2*}$ is proportional to the state-to-state gradient of the first passage times for $Fd/k_BT \ll 1$, as derived in Section V A. As noticed above, states with low ring index $m$ exhibit large ring-to-ring first passage time gradients. Thus, low-$m$ states should also exhibit a higher sensitivity. Such a correlation is confirmed in Fig. S8 (c), and this trend is also seen to hold at finite $Fd/k_BT$.

We conclude that the optimal policy close to the target tends to exhibit both a larger policy robustness and a larger relevance for the efficiency. The increased robustness to temperature changes of the policy in the most relevant states is confirmed by the observation that $\sigma[\pi_{1*}, \pi_{2*} : \chi_{2*}] > \sigma[\pi_{1*}, \pi_{2*} : 1]$ in Fig. S7 (a). This leads to an increased transferability of the optimal policy.

### A. Expansion around the optimal policy

Let us now define $\tilde{q}_\pi(s, a, \bar{s})$ as the action-value function, which provides the value taking the action $a$ in state

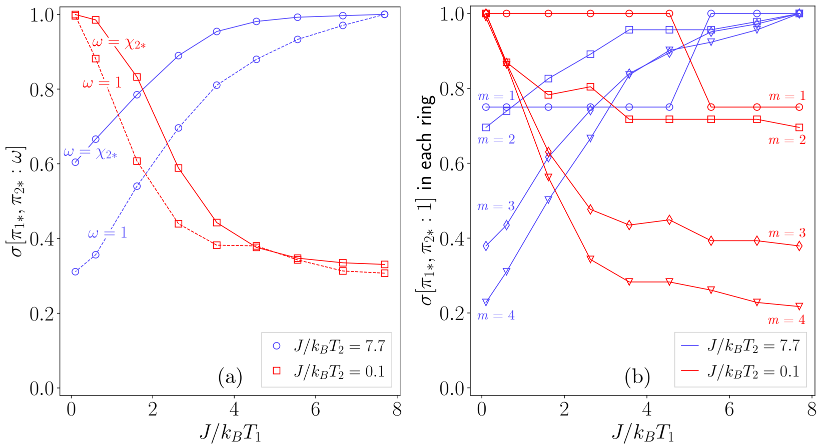


Figure S7. Transfer learning. (a) Unweighted (dashed line) and weighted (continuous line) similarities between the two optimal policies $\pi_{1*}$ at $T_1$ and $\pi_{2*}$ at $T_2$ obtained with the same value of the force $Fd/J = 0.4$, for low (blue) and high (red) temperature $T_2$. (b) Unweighted similarity in a given ring. Same parameters as in (a). Results are shown for the first rings $m = 1$ to 4.

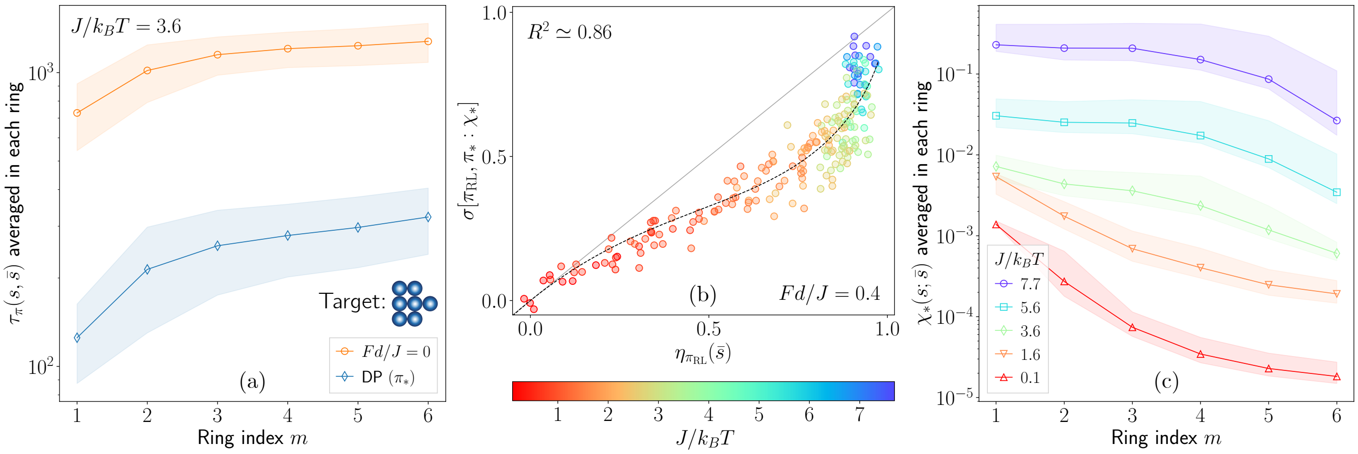


Figure S8. Analysis of transfer learning at $Fd/J = 0.4$. (a) First passage time to target averaged in each ring at $J/k_BT = 3.6$. (b) Correlation between efficiency and weighted similarity $\sigma[\pi_{\rm RL}, \pi_*, \chi_*]$ where the RL policy $\pi_{RL}$, the optimal policy $\pi_*$ and $\chi_*$ are obtained at the same temperature $T$ (dashed curve: a fit with the function $ax - bx^2\sqrt{1-x}$ leads to $a \simeq 1$, $b \simeq 1$, coefficient of determination $R^2 \simeq 0.86$). The light-gray line corresponds to a perfect equality in Eq. (54). Plots for other values of $Fd/J$ are reported in Fig. S9. (c) Sensitivity averaged in each ring for different values of $J/k_BT$. In (c) the shaded area represents the standard deviation of the points above the average sensitivity and the standard deviation of the points below it.

$s$ and then following the policy $\pi$

$$\tilde{q}_\pi(s, a; \bar{s}) = -t(s, a) - \sum_{s' \in \mathcal{B}_s} p(s'|s, a)\tau_\pi(s', \bar{s}) \,. \tag{55}$$

Expanding to linear order in $\gamma_1 - \gamma_2$, we have:

$$\begin{aligned}&\mathbb{E}_{\pi_1}[-\tilde{q}_2(s, a, \bar{s})] - \tilde{\tau}_2(s, \bar{s}) \\ &= t_2(s)\tilde{\Delta}^\dagger_{\gamma_1-\gamma_2}\tau_2(s; \bar{s}) + O(\gamma_1 - \gamma_2)^2 \,.\end{aligned} \tag{56}$$

Inserting this relation in Eq. (15) and using Eq. (13), we obtain to linear order in $\gamma_1 - \gamma_2$

$$\begin{aligned}\frac{\tau_1^\ell(\bar{s})}{\tau_2^\ell(\bar{s})} - 1 = &\sum_s \frac{\mathbb{E}_{\pi_1}[-\tilde{q}_2(s, a, \bar{s})] - \tilde{\tau}_2(s, \bar{s})}{\tau_2^\ell(s)} \\ &+ O(\gamma_1 - \gamma_2)^2 \,.\end{aligned} \tag{57}$$

Using the substitution $\pi_2 \to \pi_*$ and Eq. (30), we obtain

$$\eta^\ell_{\pi_1}(\bar{s}) = \xi_{\pi_1|\pi_*}(\bar{s}) + O(\gamma_1 - \gamma_*)^2 \,, \tag{58}$$

$$\xi_{\pi_1|\pi_*}(\bar{s}) = \sum_s \frac{\chi^\ell_{\pi_1|\pi_*}(s, \bar{s})}{\sum_{s'} \chi^\ell_{\pi_*|\pi_*}(s', \bar{s})} \,, \tag{59}$$

$$\chi^\ell_{\pi_1|\pi_2}(s, \bar{s}) = \frac{\mathbb{E}_{\pi_{\rm rand}}[\tilde{q}_2(s, a, \bar{s})] - \mathbb{E}_{\pi_1}[\tilde{q}_2(s, a, \bar{s})]}{\tau_2^\ell(s)} \,. \tag{60}$$

A numerical check, reported in Fig. S9, confirms Eq. (58) for small $\vartheta = Fd/k_BT$. Moreover, $\eta^\ell_{\pi_1}(\bar{s})$ and $\xi_{\pi_1|\pi_*}(\bar{s})$ are still correlated with a nonlinear but monotonous relation for finite $\vartheta$.

Several remarks are in order. First, Eq. (58) refers to the action-value function $q$ which is the reference quantity

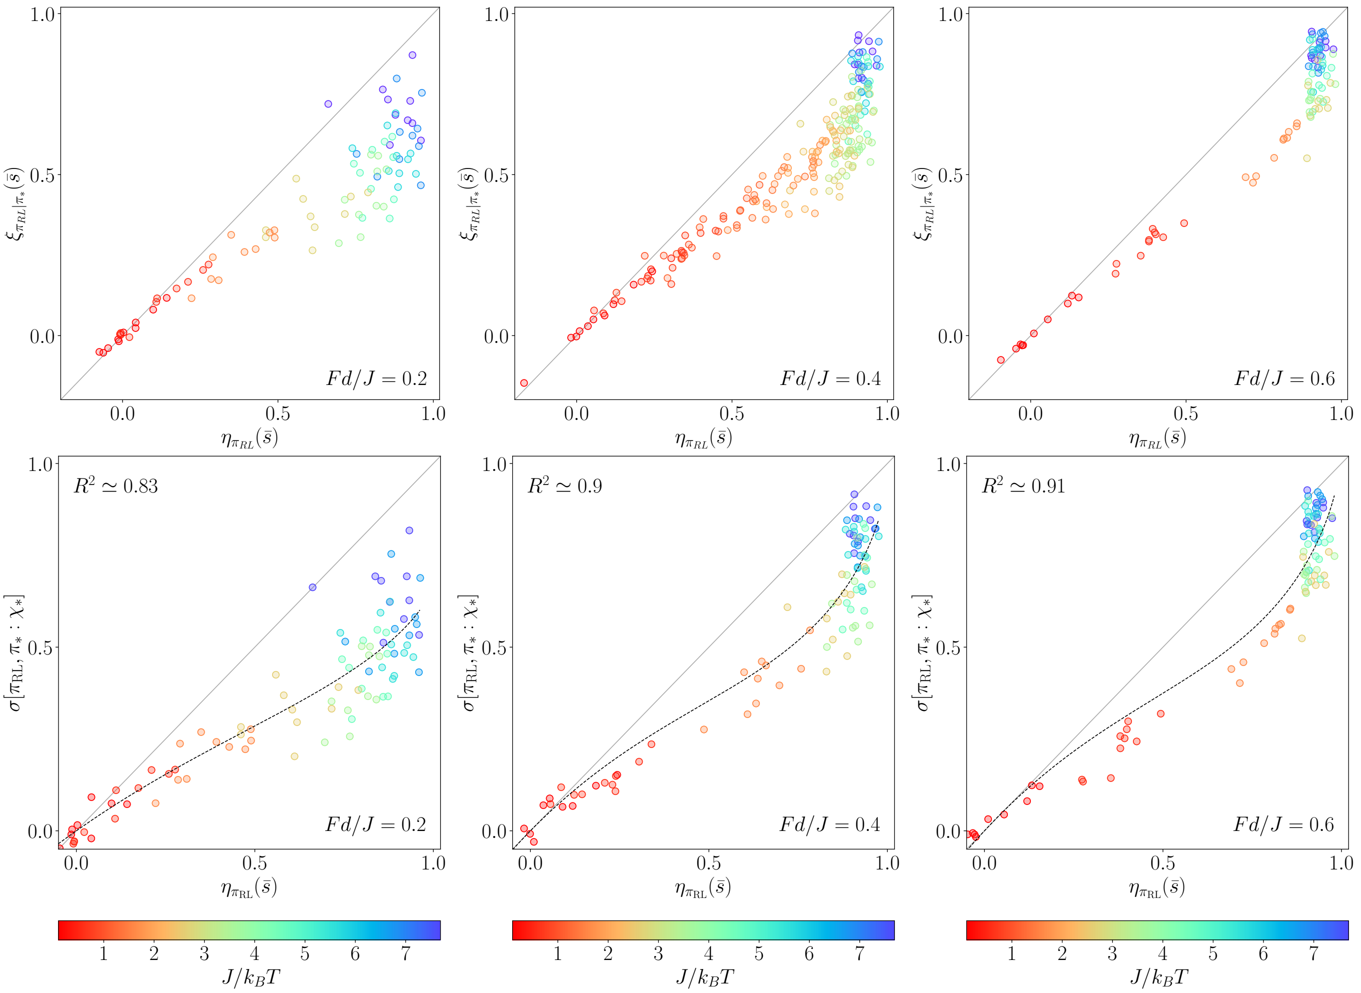


Figure S9. Top panels: correlation between learning efficiency $\eta_{\pi_{\rm RL}}(\bar{s})$ and $\xi_{\pi_{\rm RL}|\pi_*}(\bar{s})$, respectively defined in Eq. (4) of the main text and Eq. (59), for different values of $Fd/J$. Bottom panels: correlation of $\eta_{\pi_{\rm RL}}(\bar{s})$ with the weighted similarity $\sigma[\pi_{\rm RL}, \pi_*, \chi_*]$ ($\pi_{RL}$ and $\pi_*$ are obtained at the same temperature $T$). Each point corresponds to the average over 10 independent learning runs.

in the RL methods discussed in the literature [1]. Second remark, the expansion around the optimal policy, on which this relation is based, is a meaningful assumption for all $\vartheta = Fd/k_BT$. Indeed, at small $\vartheta$, all the rates are similar, while at larger $\vartheta$, the RL policies converge close to the optimal policy. Third remark, combining Eqs. (56), (20) and (60), and using the notation

$$\chi_*^\ell(s, \bar{s}) = \chi_{\pi_*|\pi_*}^\ell(s, \bar{s})$$

and the condition Eq. (32), we obtain for $\vartheta \ll 1$

$$\chi_*^\ell(s, \bar{s}) \approx -\vartheta\, P_*(s)\, \mathbf{a}_*(s) \cdot \tilde{\nabla}_{\gamma_*}^\dagger \tau_*(s; \bar{s})\,. \tag{61}$$

Hence, the sensitivity $\chi_*^\ell$ is seen to be proportional to the gradient of the optimal first passage time $\tilde{\nabla}_{\gamma_*}^\dagger \tau_*(s; \bar{s})$. This proportionality is important in the discussions of the main text. In the case with three actions along the $x$ direction considered in our simulations, we obtain

$$\chi_*^\ell(s, \bar{s}) \approx \vartheta\, P_*(s)\, |\mathbf{e}_x \cdot \tilde{\nabla}_{\gamma_*}^\dagger \tau_*(s; \bar{s})|\,. \tag{62}$$

Finally, as a fourth remark, Eq. (58) can serve as a basis for the approximate expression of the efficiency derived in the following paragraph.

### B. Linear policy interpolation

We now use an additional assumption, namely the policy in each state $s$ is assumed to interpolate linearly between a deterministic optimal policy at $\epsilon_*(s) = 0$ and a random policy at $\epsilon_*(s) = 1$:

$$\pi_{\rm lin}(a|s) = (1 - \epsilon_*(s))\pi_*(a|s) + \epsilon_*(s)\pi_{\rm rand}(a|s)\,. \tag{63}$$

The parameter $1 - \epsilon_*(s)$ can be interpreted as the advancement of learning in the state $s$. On the one hand,

we have from Eqs. (58) and (60)

$$\xi_{\pi_{\text{lin}}|\pi_*}(\bar{s}) = \sum_s (1-\epsilon_*(s)) \frac{\chi_*^\ell(s,\bar{s})}{\sum_{s'} \chi_*^\ell(s',\bar{s})} . \quad (64)$$

On the other hand, since the optimal policy is deterministic, we have $\pi_*(a|s)^2 = \pi_*(a|s)$. Hence,

$$\mathbb{E}_{\pi_{\text{lin}}}[\pi_*(a|s)] - \pi_{\text{rand}}(a|s) = (1-\epsilon_*(s)) \left(1 - \frac{1}{|\mathcal{A}|}\right) .$$

We use this expression to eliminate the dependence on $\epsilon_*(s)$ in Eq. (64). In addition, for a deterministic RL policy $\pi_{\text{RL}}$ with actions $a_{\text{RL}}(s)$, we make the heuristic substitution $\mathbb{E}_{\pi_{\text{lin}}}[\pi_*(a|s)] \to \delta_{a_{\text{RL}}(s),a_*(s)}$, leading to

$$\xi_{\pi_{\text{lin}}|\pi_*}(\bar{s}) = \sum_s \frac{\delta_{a_{\text{RL}}(s),a_*(s)} - 1/|\mathcal{A}|}{1-1/|\mathcal{A}|} \frac{\chi_*(s,\bar{s})}{\sum_{s'} \chi_*(s',\bar{s})} . \quad (65)$$

Combining this relation with Eq. (58), and using the substitution $\chi_*^\ell \to \chi_*$ leads to Eq. (54).


[1] R. S. Sutton and A. G. Barto, *Reinforcement Learning: An Introduction*, 2nd ed. (The MIT Press, 2018).

[2] F. Boccardo, Y. Benamara, and O. Pierre-Louis, Phys. Rev. E **106**, 024120 (2022).

[3] N. G. Van Kampen, *Stochastic processes in physics and chemistry* (Elsevier, 1992).

[4] M. Kac, Bulletin of the American Mathematical Society **53**, 1002 (1947).

[5] F. Boccardo and O. Pierre-Louis, Phys. Rev. Lett. **128**, 256102 (2022).

[6] A. Baronchelli and V. Loreto, Phys. Rev. E **73**, 026103 (2006).
